# Supplementary material for: On the preparation and NMR spectroscopic characterization of potassium aluminium tetrahydride KAlH4
Source: arXiv:1902.08540 ancillary file (2019-08-22)
Supplement: Supplementary file 1 [file KAlH4_ESI_ref.pdf]

# On the preparation and NMR spectroscopic characterization of potassium aluminium tetrahydride $\text{KAlH}_4$

Bodo Zibrowius and Michael Felderhoff

*Max-Planck-Institut für Kohlenforschung,*

*Kaiser-Wilhelm-Platz 1, 45470 Mülheim an der Ruhr, Germany*

*E-mail: [zibrowius@mpi-muelheim.mpg.de](mailto:zibrowius@mpi-muelheim.mpg.de), [felderhoff@mpi-muelheim.mpg.de](mailto:felderhoff@mpi-muelheim.mpg.de)*

**Note:** For the sake of transparency, we have included the complete reviewer reports and our answers. We feel that these reports exemplify the paramount importance of the current refereeing system for maintaining the outstanding scientific level of a high-ranking journal in physical chemistry.

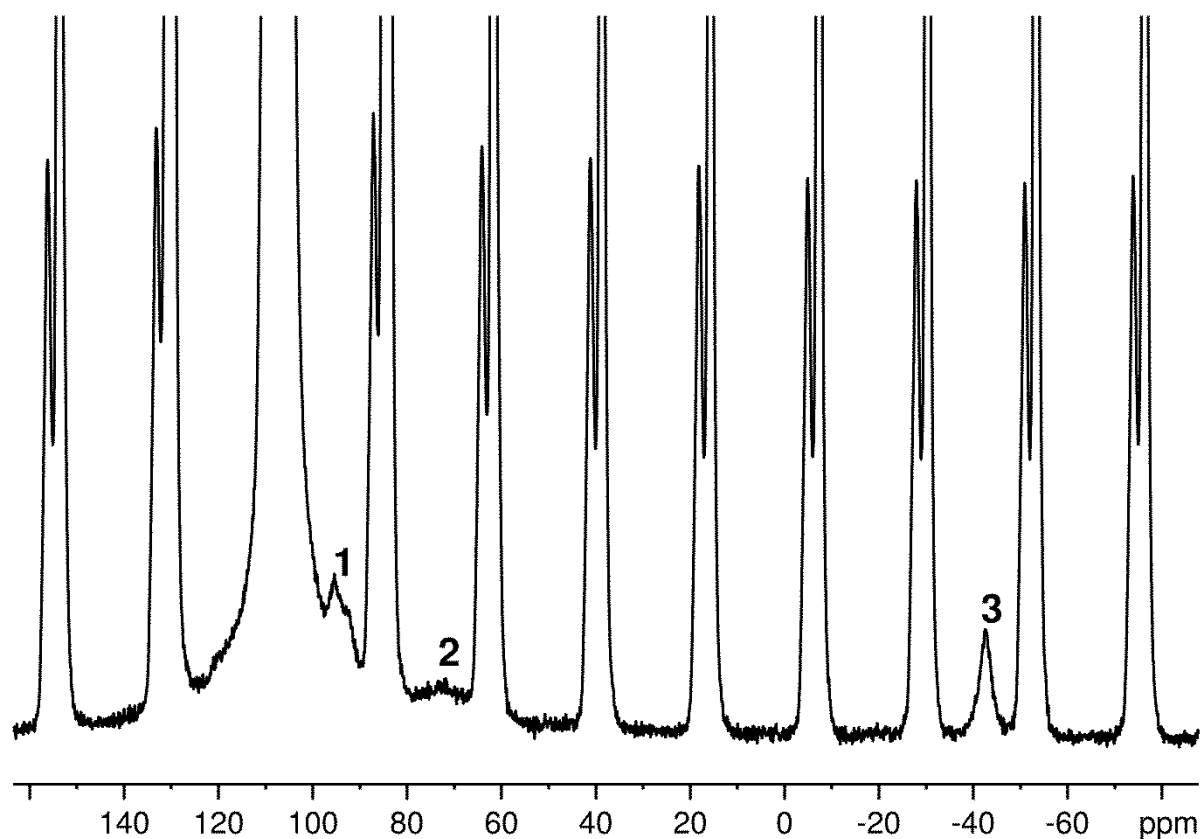

**Fig. S1**  $^{27}\text{Al}$  MAS NMR spectrum of  $\text{KAlH}_4$  measured at  $\nu_{\text{MAS}} = 3$  kHz as in Fig. 2, but here enlarged to show the resonance lines due to impurities present: (1)  $\text{NaAlH}_4$ , (2) aluminium oxide, and (3)  $\text{Na}_3\text{AlH}_6$ . To estimate the amount of by-products one can use the intensity of the visible spinning sidebands of the  $\text{KAlH}_4$  outer satellite transition that amounts to about 6‰ of the intensity of the centreband of the central transition. Hence, all aluminium containing by-products are traces in the per mille range.

**Table S1** Parameters used to simulate the  $^{27}\text{Al}$  MAS NMR sideband patterns shown in Fig. 4, Fig. S2 and Fig. S3 by means of the solids lineshape analysis module implemented in the TopSpin<sup>TM</sup> 3.2 NMR software package

| Parameter                  | Value       |
|----------------------------|-------------|
| TRIANG                     | 64          |
| Model                      | QUAD all    |
| MASR                       | 1400 / 3000 |
| Angle                      | 54.7        |
| Side bands                 | 278 /131    |
| $\delta(\text{iso})$ [ppm] | 107.6       |
| CQ(Quad) [kHz]             | 1290        |
| $\eta(\text{Quad})$        | 0.64        |
| LB                         | 60          |
| GB                         | 120         |

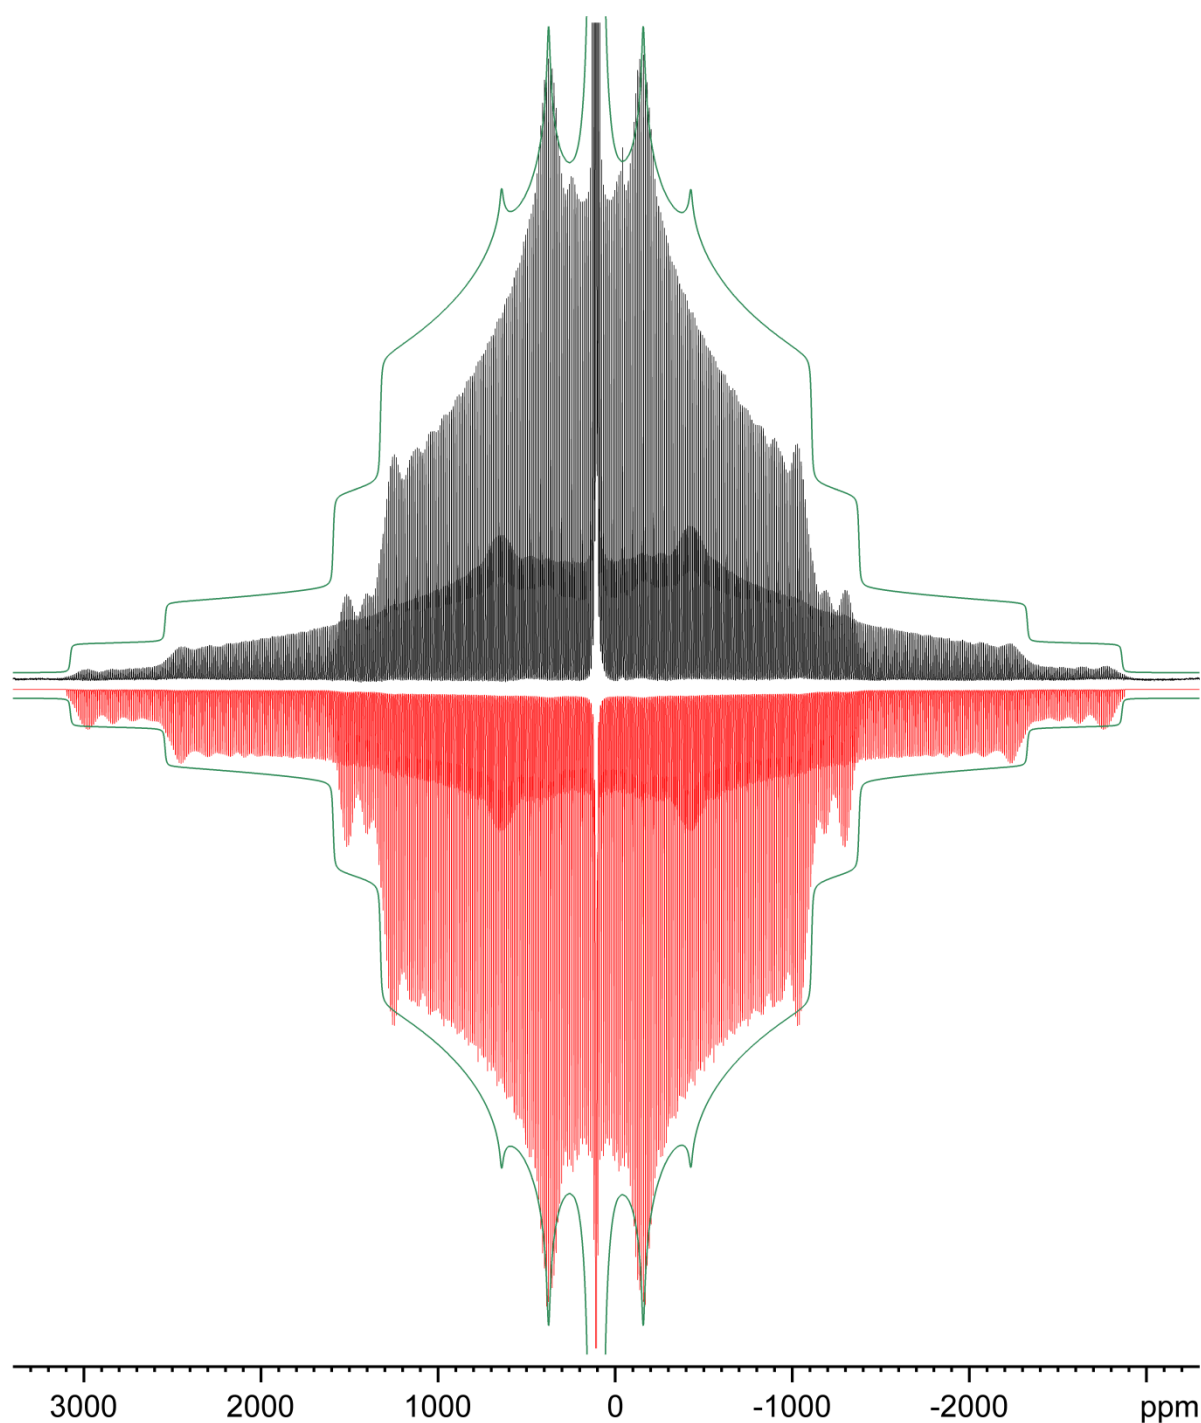

**Fig. S2** Experimental  $^{27}\text{Al}$  MAS NMR spectrum of  $\text{KAlH}_4$  measured at  $\nu_{\text{MAS}} = 1.4$  kHz (black) and its simulation (red) with the parameters  $\delta_{\text{iso}} = 107.6$  ppm,  $C_Q = 1.29$  MHz and  $\eta = 0.64$ . To ease the comparison, the simulated MAS NMR spectrum has been inverted. The green lines depict the lineshape one would obtain for a non-spinning sample.

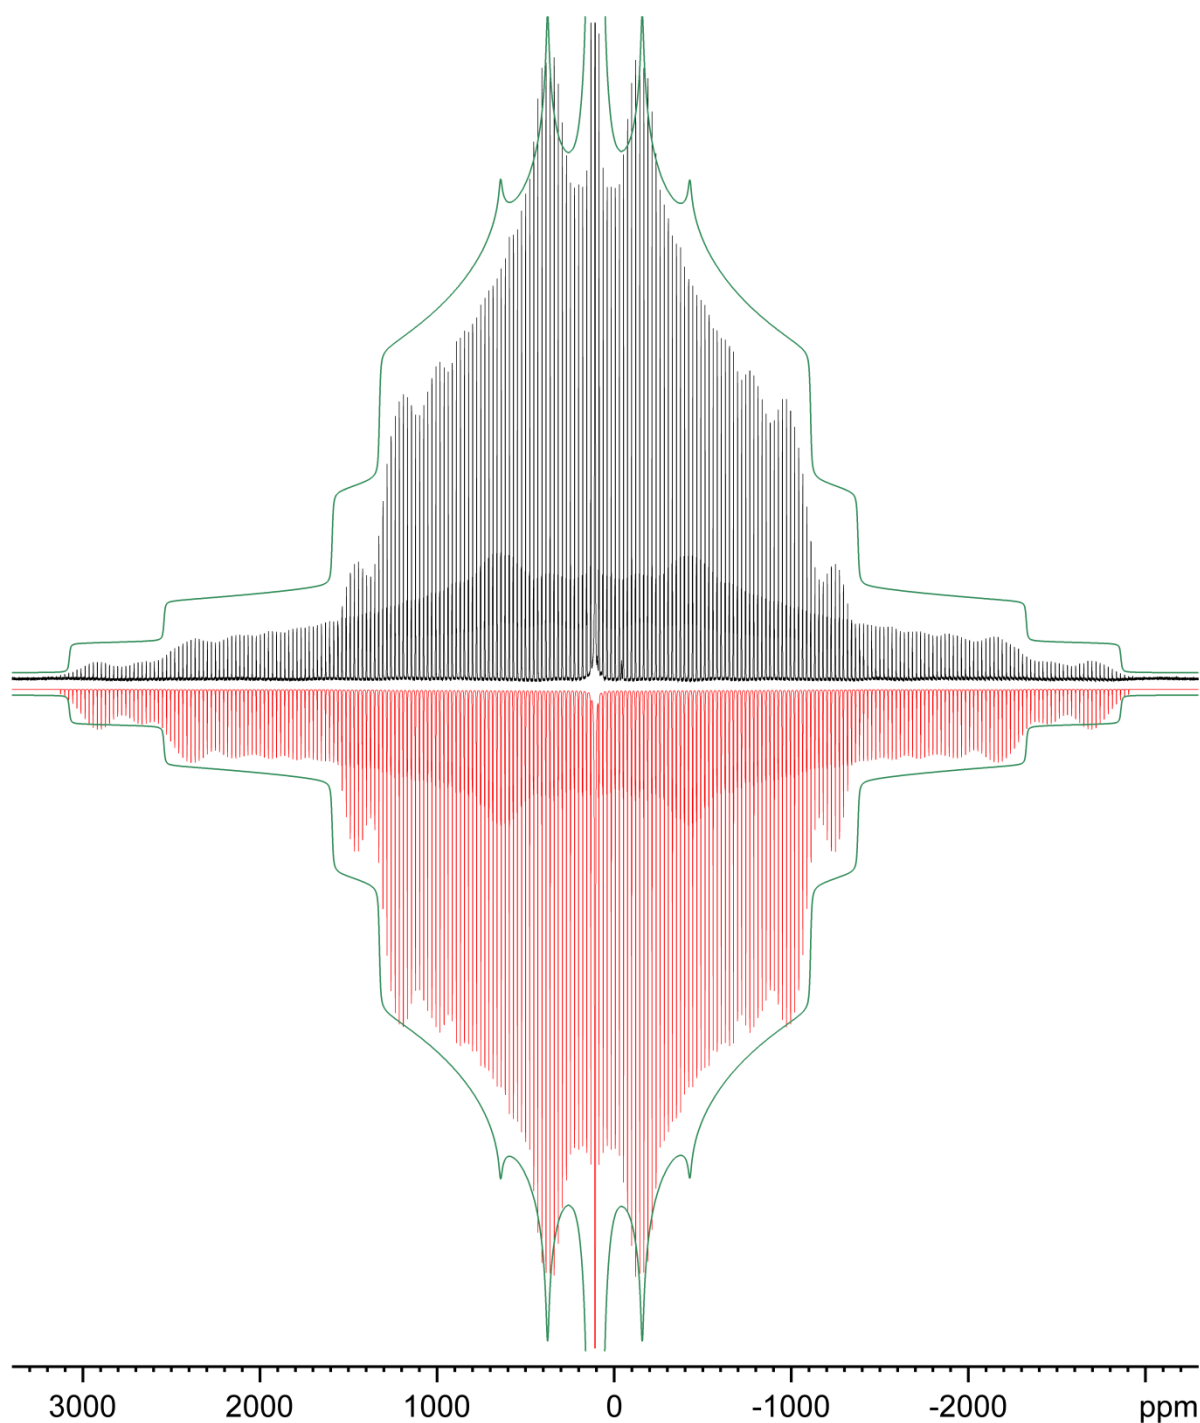

**Fig. S3** Experimental  $^{27}\text{Al}$  MAS NMR spectrum of  $\text{KAlH}_4$  measured at  $\nu_{\text{MAS}} = 3.0$  kHz (black) and its simulation (red) with the parameters  $\delta_{\text{iso}} = 107.6$  ppm,  $C_Q = 1.29$  MHz and  $\eta = 0.64$ . To ease the comparison, the simulated MAS NMR spectrum has been inverted. Again, the green lines depict the lineshape one would obtain for a non-spinning sample.

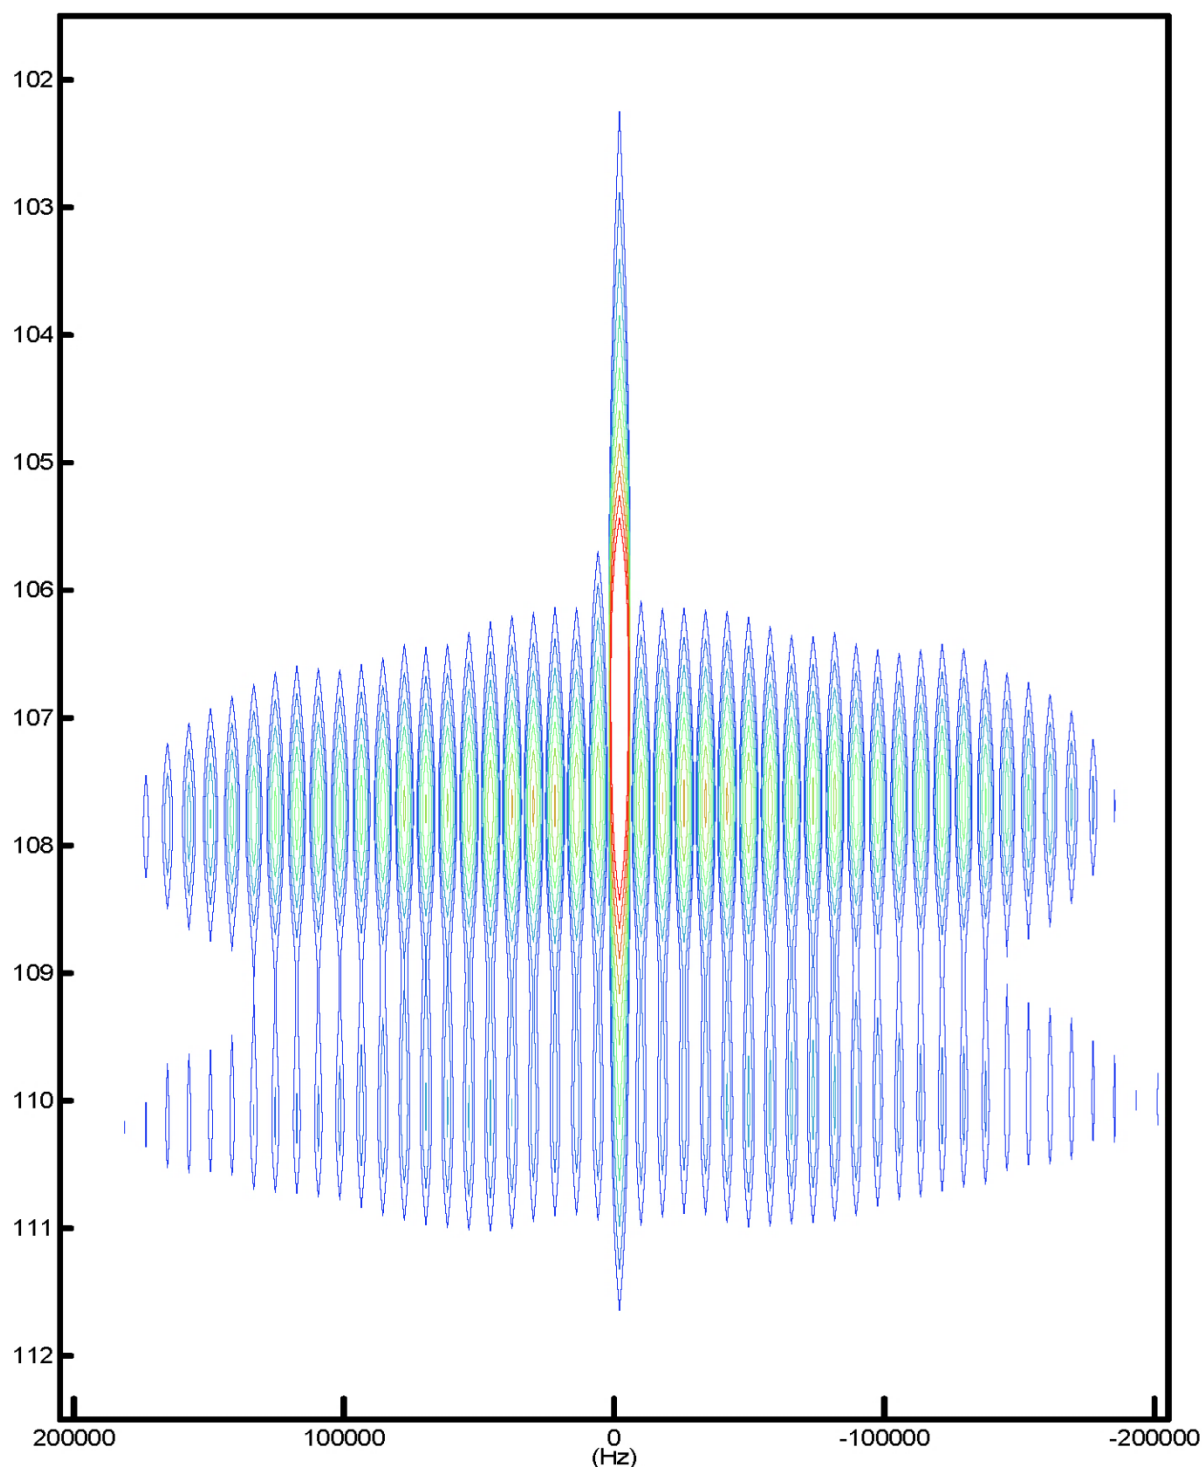

**Fig. S4**  $^{27}\text{Al}$  TOP NMR spectrum of  $\text{KAlH}_4$ . This spectrum is just a different presentation of the MAS NMR spectrum ( $\nu_{\text{MAS}} = 8$  kHz) given in Fig. 3. Following the suggestion of one of the referees, we have used the software package dmfit (D. Massiot et al., *Magn. Reson. Chem.* 40 (2002) 70-76; dmfit/x64/release#20190125; available from: [nmr.cemhti.cnrs-orleans.fr](http://nmr.cemhti.cnrs-orleans.fr)) to process the data recorded. The positions of the resonance lines of the different transitions can directly be read out from this plot. These values are slightly lower than those given in the text as derived from the spectrum measured at  $\nu_{\text{MAS}} = 3$  kHz. The small shift is due to frictional heating at higher spinning frequencies as mentioned in the paper.

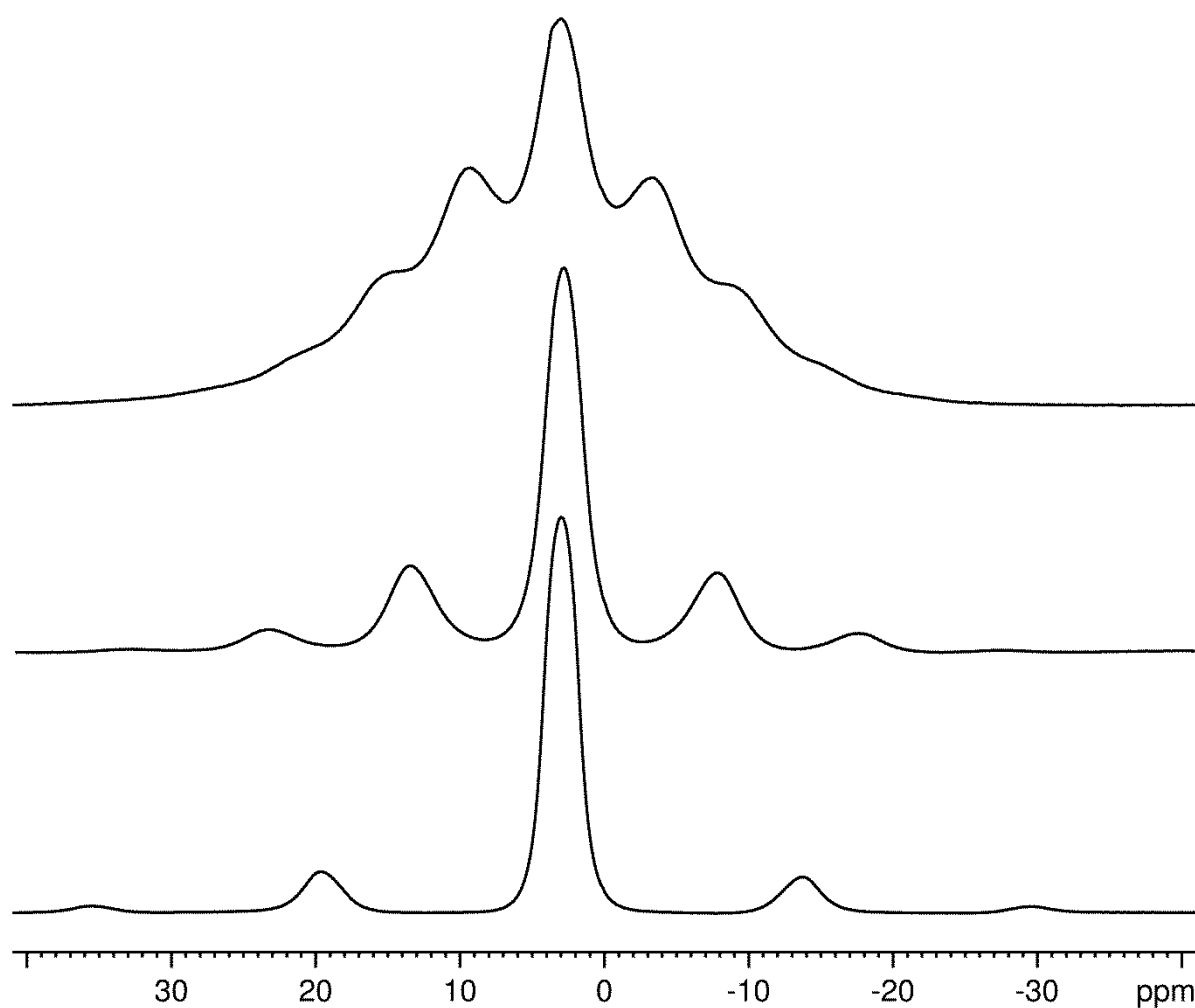

**Fig. S5**  $^1\text{H}$  MAS NMR spectra of  $\text{KAlH}_4$  recorded at different spinning frequencies  $\nu_{\text{MAS}}$ : 3 kHz (top), 5 kHz (middle), and 8 kHz (bottom). The experimental conditions are as follows: 500 MHz resonance frequency, 10 s repetition delay, and  $3.0\ \mu\text{s}\ \pi/4$  pulses. At  $\nu_{\text{MAS}} = 8\ \text{kHz}$ , the full width at half height of the line at 2.95 ppm amounts to about 1.3 kHz. The spectra give no indication of the presence of by-products.

## REVIEWER REPORTS

Referee: 1

Comments to the Author

PCCP wants to publish papers that have high quality work and give significant new physical insights.

A sample in this pure phase loses all applicability to “real” systems, and so seems inapplicable when the reason KAlH<sub>4</sub> is interesting at all is for its potential in hydrogen storage (as stated explicitly in the abstract of this manuscript). In that application, one would not be encountering pure phase or even chemically pure at all (for that matter) material. So to focus so on the pure material and pure phase is mostly of intellectual pure scientific interest, remote from the application that makes it interesting to more people than just a few.

I think this work should be published in a suitable SSNMR journal that sees recording structural parameters of pure materials as its goal. This paper does that very well with high quality.

On the final page, just above the conclusions, the authors make a comment about the 39K resonance observed in a 2014 paper on an unannealed KAlH<sub>4</sub> sample. The statement is "we have to conclude that the 39K NMR line reported by Sorte et al is not caused by the potassium ions in Pnma KAlH<sub>4</sub>." To me this sounds as if the authors are suggesting that this resonance came from something else in the probe (a very unlikely idea, given the extremely low sensitivity of 39K). I would rephrase that sentence to say "the signals reported by Sorte et al are clearly affected by the other phases of KAlH<sub>4</sub> present in their sample." This is probably closer to what was meant and what is likely true.

Referee: 2

Comments to the Author

Comments to manuscript untitled “On the preparation and NMR spectroscopic characterization of potassium aluminium tetrahydride KAlH<sub>4</sub>” by B. Zibrowius et al.

During last decade, the alanates have been occupied a remarkable place into the hydrogen storage materials and, moreover they have important given clues about the hydrogenation mechanism of other complex hydrides. In this work, authors present an exhaustive investigation about the NMR characterization of potassium alanate. This compound has been barely investigated compared to the well-known alkaline alanates (Li, Na) but, contrary to those, it exhibits an easy H-reversibility at moderate temperatures and pressures. Therefore, KAlH<sub>4</sub> is an excellent playground to investigate the formation/desorption process to obtain useful information that could be used in more complex alanates.

The work is very exhaustive being particularly interested to the hydrogen community. Authors synthesise KAlH<sub>4</sub> by metathesis method and it is characterized by NMR and XRD. The work reveals that 27Al could be considered a blueprint and could be extended to other (and more complex) alanates. It fits into the PCCP journal and I recommend its publication after next clarification

Preparation of KAlH<sub>4</sub> is performed by metathesis. This synthesis could leave undesirable products. Have authors observed some “impurity” after preparation in the alanate? XRD seems to show a broad peak about 20-22°. Could be attributed to an amorphous phase? Authors should explain this XRD feature.

Referee: 3

#### Comments to the Author

This paper presents a very detailed and well conducted NMR analysis of a well crystallized and purified KAlH<sub>4</sub> sample. The Authors obtain, for the first time, unambiguous set of NMR parameters of <sup>27</sup>Al (single site according the X-ray structure) which contrasts to previous studies where either several values were reported or the lack of well defined quadrupolar features, ascribed to a disorder resulting from the synthesis route (ball-milling), was outlined.

The determination of the NMR parameters is based on a detailed analysis of the Spinning Sidebands manifold of the satellite transitions as the quadrupolar coupling is too small to provide a resolved second-order quadrupolar broadening lineshape. This is a rather well established approach in NMR methodology for such situation. However, given the importance of NMR for hydride studies, based on the quality of the data obtain, I would support a publication in PCCP.

I have however few comments :

#### - NMR experiments

Was a <sup>1</sup>H decoupling necessary ? (or detrimental to the resolution) Should be explicitly mentioned. <sup>1</sup>H NMR data should be presented. They are reported in Ref. 24 and it would be interesting to see if some difference exists, as well as to verify the absence of KH peaks.

Only the total spinning sidebands manifolds is given. I would recommend the authors to display the individual spinning sidebands (as the inner and outer ST transitions are resolved, see Fig.2 are resolved).

I would also recommend the authors to present their data with co-added spinning sideband (TOP see REF D.Massiot, et 'Two dimensional One Pulse MAS of Half-Integer Quadrupolar Nuclei' Journal of Magnetic Resonance 181 310-315 (2006) This should provide an alternative and reliable method to determine the quadrupolar parameters from the ST positions.

Why no MQMAS ? The shape of the Al line in the 2D spectrum should be able to reveal if a residual disorder persists.

I regret that the authors did compare their experimental NMR parameters with DFT calculations, as the GIPAW method is routinely applied (and simple to use) in the field and was found to provide reliable NMR parameters for other phases (see. Ref 15).

KAlH<sub>4</sub> is known to be reactive without the need of any catalyst. Here the authors do not report any data about the reactivity of their sample. As the quality of the NMR spectra (resolution) suggests a high purity phase and well ordered system observed in the present work, It would have been interesting to have such data to compare their sample to standard ones. The point is to know whether disorder or impurities can explain the high reactivity of KAlH<sub>4</sub> in previous studies. Maybe some comment in this point should be added.



## Answers to the referees

### Referee 1:

We oppose almost any statement made by referee 1.

In particular, we reply the following:

*"A sample in this pure phase loses all applicability to "real" systems, and so seems inapplicable when the reason KAlH<sub>4</sub> is interesting at all is for its potential in hydrogen storage (as stated explicitly in the abstract of this manuscript)."*

(i) To regard a material that has been obtained by recrystallization after salt metathesis as too pure to be applicable to "real" systems is preposterous. Ref. 31 is a perfect example how pointless investigations of ill-defined materials without comparison to well-defined reference materials are.

(ii) There is no statement about potassium alanate as potential hydrogen storage material in the abstract of our manuscript. We even state in the Introduction that "KAlH<sub>4</sub> is of course a rather unlikely candidate for a widespread application as hydrogen storage material." Either some degree of reading disability or a certain amount of bad intent is necessary to misunderstand our clear statement.

*"On the final page, just above the conclusions, the authors make a comment about the 39K resonance observed in a 2014 paper on an unannealed KAlH<sub>4</sub> sample. The statement is "we have to conclude that the 39K NMR line reported by Sorte et al is not caused by the potassium ions in Pnma KAlH<sub>4</sub>." To me this sounds as if the authors are suggesting that this resonance came from something else in the probe (a very unlikely idea, given the extremely low sensitivity of 39K). I would rephrase that sentence to say "the signals reported by Sorte et al are clearly affected by the other phases of KAlH<sub>4</sub> present in their sample." This is probably closer to what was meant and what is likely true."*

The referee is totally wrong. We want to say *"that this resonance came from something else in the probe."* One of us happened to be a referee of ref. 31 and has seen the appalling xrd pattern of the unannealed sample that was originally part of the paper. In the published paper, the authors report: The pattern "showed several peaks that do not correspond to Pnma KAlH<sub>4</sub>. These peaks could be due to unknown impurities or other crystal phases of KAlH<sub>4</sub>." Hence, our statement is perfectly justified.

Conclusion: No action required.

### Referee 2:

We thank the referee for the positive report.

As regards the "broad peak about 20-22°", we feel that the vast majority of the readers of PCCP, especially those who are dealing with solids and their characterisation, are fully aware of the origin of this peak. Under Experimental, we clearly state that the sample was measured in a glass capillary.

Conclusion: No action required.

### Referee 3:

We want to thank the referee for his positive and very detailed report.

*Was a  $^1\text{H}$  decoupling necessary ? (or detrimental to the resolution) Should be explicitly mentioned.*

The suspicion by the referee is justified. Proton decoupling is not really necessary to achieve the resolution we got. At spinning speeds above about 5 kHz the influence is hardly visible. To keep the experimental conditions as similar as possible to those of our earlier study on caesium alanates (ref. 32) we used proton decoupling for all spectra. We added a remark concerning the influence of decoupling (see Experimental).

*$^1\text{H}$  NMR data should be presented. They are reported in Ref. 24 and it would be interesting to see if some difference exists, as well as to verify the absence of KH peaks.*

Although we think that  $^1\text{H}$  MAS NMR spectra do not contribute much to the characterisation of complex aluminium hydrides, we have added Fig. S5 to the ESI. This figure shows spectra taken at different spinning speeds. As expected, there is no indication of the presence of any KH. According to our experience, KH is difficult to be missed in the xrd pattern. The resonance line of  $\text{KAlH}_4$  at about 3 ppm (FWHH = 1.3 kHz at a spinning speed of 8 kHz) is very similar to that obtained in ref. 24. We have added a remark concerning the  $^1\text{H}$  MAS NMR spectra in Fig. S5 at the end of the “ $^{27}\text{Al}$  MAS NMR spectroscopy”.

*Only the total spinning sidebands manifolds is given. I would recommend the authors to display the individual spinning sidebands (as the inner and outer ST transitions are resolved, see Fig.2 are resolved).*

We do not fully understand what the referee wants us to do. The resolution of the sidebands of the satellite transitions is evident from Figs 2 and S1. The two sets of sideband patterns can also be discerned in Figs S2 and S3.

*I would also recommend the authors to present their data with co-added spinning sideband (TOP see REF D.Massiot, et 'Two dimensional One Pulse MAS of Half-Integer Quadrupolar Nuclei' Journal of Magnetic Resonance 181 310-315 (2006) This should provide an alternative and reliable method to determine the quadrupolar parameters from the ST positions.*

We have added Fig. S4 to the ESI. It presents the spectrum shown in Fig. 3c after processing it according to the suggestion of the referee. The figure is not as impressive as the examples given by Massiot et al. Since all transitions are lacking any significant second-order line broadening, Fig. S4 is not more informative than Fig. 2. Nevertheless, we want to thank the referee for mentioning this alternative. We have also added a remark to the text (see paragraph after eqn 10).

*Why no MQMAS ? The shape of the Al line in the 2D spectrum should be able to reveal if a residual disorder persists.*

MQMAS is of course an alternative approach to obtain the parameters we derived. It was one of the main objectives of our paper to demonstrate that a wealth of information can be derived from conventional 1D NMR spectra. We adhere to the KISS principle. Furthermore, we do not think that the accuracy of data derived from MQMAS would be superior. For more reactive samples, we would even recommend the application of Solomon echoes on stationary samples as mentioned in the paper as alternative approach.

*I regret that the authors did compare their experimental NMR parameters with DFT calculations, as the GIPAW method is routinely applied (and simple to use) in the field and was found to provide reliable NMR parameters for other phases (see. Ref 15).*

We agree that the comparison with calculated data would be a natural thing to include and we would love to do so. However, we do not have the necessary expertise to perform those calculations and to judge the significance of their results. With the nowadays widespread availability of suitable equipment, a lot of people with little or no expertise in solid-state NMR undertake the endeavour to perform measurements and to interpret the outcome with sometimes rather funny conclusions (e. g. discovery of “NMR invisible phosphorous” in analogy to “NMR invisible aluminium” in Chem. Mater. 2005, 17, 3921). We do not want to end up in a similar situation by entering a field of science we are totally unfamiliar with. We leave the comparison to the experts.

*KAlH<sub>4</sub> is known to be reactive without the need of any catalyst. Here the authors do not report any data about the reactivity of their sample. As the quality of the NMR spectra (resolution) suggests a high purity phase and well ordered system observed in the present work, It would have been interesting to have such data to compare their sample to standard ones. The point is to know whether disorder or impurities can explain the high reactivity of KAlH<sub>4</sub> in previous studies. Maybe some comment in this point should be added.*

To study the reactivity of KAlH<sub>4</sub> is far beyond the goals of our paper. Although we agree that the presence of defects might have an influence on dehydrogenation properties we want to refrain from speculations.
